# Supplementary material for: System Resilience through Health Monitoring and Reconfiguration
Source: arXiv:2208.14525 source file (2022-08-30)
Supplement: Supplementary file 1 [file appendix.tex]

\clearpage
\appendix
\section{Appendix}
\subsection{Tables of input, output and fault parameter names}
\begin{table}[htp!]
\small
\centering
\begin{tabular}{|c|c|}\toprule
\textbf{Input name} & \textbf{Description} \\\midrule
reference\_1 & controls the volumetric rate of pump 1\\  \midrule
reference\_2 & controls the volumetric rate of pump 2\\  \midrule
control\_valve\_6 & controls the opening of valve 6\\  \midrule
control\_valve\_7 & controls the opening of valve 7\\  \midrule
control\_valve\_8 & controls the opening of valve 8\\  \midrule
control\_valve\_9 & controls the opening of valve 9\\  \midrule
control\_valve\_10 & controls the opening of valve 10\\  \midrule
control\_valve\_11 & controls the opening of valve 11\\  \midrule
control\_valve\_12 & controls the opening of valve 12\\  \midrule
control\_valve\_13 & controls the opening of valve 13\\  \midrule
control\_valve\_14 & controls the opening of valve 14\\  \midrule
control\_valve\_15 & controls the opening of valve 15\\  \midrule
control\_valve\_16 & controls the opening of valve 16\\  \bottomrule
\end{tabular}
\caption{Input names and descriptions}\label{tab:input names}
\end{table}

\begin{table}[htp!]
\small
\centering
\begin{tabular}{|c|c|}\toprule
\textbf{Output name} & \textbf{Description} \\\midrule
massFlow\_1 & mass flow rate at tank 1\\  \midrule
massFlow\_2 & mass flow rate at tank 2\\  \midrule
massFlow\_3 & mass flow rate at pipe 1\\  \midrule
massFlow\_4 & mass flow rate at pipe 2\\  \midrule
massFlow\_5 & mass flow rate at pipe 7\\  \midrule
massFlow\_6 & mass flow rate at pipe 6\\  \midrule
massFlow\_7 & mass flow rate at engine 1\\  \midrule
massFlow\_8 & mass flow rate at engine 2\\  \midrule
pressure\_3 & pressure at pipe 1\\  \midrule
pressure\_4 & pressure at pipe 2\\  \midrule
pressure\_5 & pressure at pipe 7\\  \midrule
pressure\_6 & pressure at pipe 6\\  \midrule
pressure\_7 & pressure at engine 1\\  \midrule
pressure\_8 & pressure at engine 2\\ \bottomrule
\end{tabular}
\caption{Output names and descriptions}\label{tab:output names}
\end{table}

\begin{table}[htp!]
\small
\centering
\begin{tabular}{|c|c|}\toprule
\textbf{Fault parameter name} & \textbf{Description} \\\midrule
leak\_fault\_1 &  magnitude of pipe 2 leak\\  \midrule
leak\_fault\_2 &  magnitude of pipe 1 leak\\  \midrule
leak\_fault\_3 & magnitude of valve 6 leak\\  \midrule
leak\_fault\_4 & magnitude of valve 7 leak\\  \midrule
leak\_fault\_5 & magnitude of pipe 6 leak\\  \midrule
leak\_fault\_6 & magnitude of pipe 7 leak\\  \midrule
leak\_fault\_7 & magnitude of pipe 10 leak\\  \midrule
leak\_fault\_8 & magnitude of pipe 11 leak\\  \midrule
stuckAt\_valve\_6 & stuck input for valve 6\\ \midrule
stuckAt\_valve\_7 & stuck input for valve 7\\ \midrule
stuckAt\_valve\_8 & stuck input for valve 8\\ \midrule
stuckAt\_valve\_9 & stuck input for valve 9\\ \midrule
stuckAt\_valve\_10 & stuck input for valve 10\\ \midrule
stuckAt\_valve\_11 & stuck input for valve 11\\ \midrule
stuckAt\_valve\_12 & stuck input for valve 12\\ \midrule
stuckAt\_valve\_13 & stuck input for valve 13\\ \midrule
stuckAt\_valve\_14 & stuck input for valve 14\\ \midrule
stuckAt\_valve\_15 & stuck input for valve 15\\ \midrule
stuckAt\_valve\_16 & stuck input for valve 16\\ \bottomrule
\end{tabular}
\caption{Fault parameter names and descriptions}\label{tab:fault names}
\end{table}
